# Supplementary material for: Glueability of resource proof-structures: inverting the Taylor expansion (long version)
Source: arXiv:1910.07936 source file (2019-10-17)
Supplement: Supplementary file 1 [file proof-nets-appendix.tex]

\section{Graphs}
\label{subsec:graphs}

We follow the definition of a graph given by \cite{Borisov2008}: in particular,
a graph is not the datum of a set of edges and a set of vertices, but the edges
are split in halves, allowing for some of them to be hanging.
\begin{definition}[graph]
  \index{graph}
  \index{flag}
  \index{vertex}
  \index{tail}
  \index{edge}
  A (finite) \emph{graph} $\tau$ is a quadruple
  $(F_{\tau}, V_{\tau}, \partial_{\tau}, j_{\tau})$, where
  \begin{itemize}
  \item $F_{\tau}$ is a finite set, whose elements are called \emph{flags} of
    $\tau$;
  \item $V_{\tau}$ is a finite set, whose elements are called \emph{vertices} of
    $\tau$;
  \item $\partial_{\tau} : F_{\tau} \to V_{\tau}$ is a function associating to
    each flag its \emph{boundary};
  \item $j_{\tau} : F_{\tau} \to F_{\tau}$ is an involution.
  \end{itemize}
\end{definition}

A flag that is fixed point of the involution $j_F$ is a \emph{tail} of $\tau$.
%Two-element orbits of $j_F$ form a set $E_{\tau}$ of \emph{edges} of
%$\tau$. Elements of an edge $e$ are called \emph{halves} of $e$.
A two-element orbit $\{f,f'\}$ of $j_F$ is an \emph{edge} of
$\tau$ between $\partial_{\tau}(f)$ and $\partial_{\tau}(f')$, and $f$ and $f'$ are the \emph{halves} of such an edge.
The set of edges of $\tau$ is denoted by $E_{\tau}$.

Given two graphs $\tau$ and $\tau'$, it is always possible to consider their
disjoint union $\tau \sqcup \tau'$ defined as the disjoint union of the
underlying sets and functions.

\index{corolla}
A one vertex graph with set of flags $F$ and involution the identity on $F$ is
called the \emph{corolla} with set of flags $F$. It is usually written
$\ast_F$. One corolla $\ast_{\mathbf{5}}$ is depicted Figure \ref{fig:corolla5}.

Given a graph $\tau = (F_{\tau}, V_{\tau}, \partial_{\tau}, j_{\tau})$, a vertex
$v$ defines a corolla $\tau_{v}$, by, if we set $F_v = \partial_{\tau}^{-1}(v)$:
\begin{align*}
  \tau_v = (F_v, \{v\}, \partial_{\tau}|_{F_v}, \id_{F_v}).
\end{align*}
Every graph can be described as the set of corollas of its vertices, together
with the involution glueing the flags in edges.

Different notions of morphisms exist between graphs. As we will be interested in
isomorphisms and subgraphs, we will use the most naive notion.

\begin{definition}[graph morphism]
  Let $\tau, \sigma$ be two graphs. A \emph{graph morphism}
  \begin{align*}
    h \colon \tau \to \sigma
  \end{align*}
  from $\tau$ to $\sigma$ is a couple of functions $(h_F \colon F_{\tau} \to F_{\sigma}, h_V \colon V_{\tau} \to
  V_{\sigma})$ such that $h_V \circ \partial_{\tau} = \partial_{\sigma} \circ
  h_F$ and $h_F \circ j_{\tau} = j_{\sigma} \circ h_F$.

  A graph morphism is \emph{injective} if %both
  its component functions are.
  A graph $\sigma$ is a \emph{subgraph} of a graph $\tau$ if there is an injective graph morphism from $\sigma$ to $\tau$.
  A graph \emph{isomorphism} is a graph morphism whose component functions are bijections.
  Graphs are identified up to isomorphism.
\end{definition}

The category $\Graph$ \index{$\Graph$} has graphs as objects and morphisms of
graphs as morphisms: indeed, graph morphisms compose (by composing the
underlying functions) and the couple of identities (on vertices and flags) is
neutral. It is a monoidal category, with disjoint union as a monoidal product.

\subsection{Graphs with structure}

Some structure can be put on top of a graph $\tau = (F_\tau, V_\tau, \partial_\tau, j_\tau)$. For instance:
\begin{definition}
  \label{def:labelled-graphs}
  \begin{itemize}
  \item A \emph{labelled graph} $(\tau,\ell_\tau)$ with labels in $I$ is a graph
    $\tau$ together with a function $\ell_\tau \colon V_{\tau} \to I$;
  \item a \emph{colored graph} $(\tau,\FlagType_\tau)$ with colors in a set $C$
    is a graph $\tau$ together with a function $\FlagType_\tau \colon F_{\tau} \to C$
    such that, for two halves $f,f'$ of any edge of $\tau$,
    \begin{align*}
      \FlagType_\tau(f) = \FlagType_\tau(f');
    \end{align*}
  \item an \emph{oriented graph} $(\tau, \Orient_\tau)$ is a graph $\tau$
    together with a function $\Orient_\tau \colon F_{\tau} \to \{\In, \Out\}$ such that,
    for two halves $f,f'$ of any edge of $\tau$,
    \begin{align*}
      \Orient_\tau(f) \neq \Orient_\tau(f');
    \end{align*}
    we then say that $\{f,f'\}$ is an edge of $\tau$ from $\partial_{\tau}(f)$ to $\partial_{\tau}(f')$;
    $\In$-oriented tails of $\tau$ are called \emph{inputs} of $\tau$,
    $\Out$-oriented tails are called \emph{outputs} of $\tau$.

   	If $v$ is a vertex of $\tau$, its \emph{inputs} are the
    elements of the set
    $\In_{\tau}(v) = \partial_{\tau}^{-1}(v) \cap \mathsf{o}^{-1}(\In)$; 
    its \emph{outputs} are the elements of the set
    $\Out_{\tau}(v) = \partial_{\tau}^{-1}(v) \cap \mathsf{o}^{-1}(\Out)$;
  \item an \emph{ordered graph} $(\tau,\leqslant_{\tau})$ is a graph together
    with an order on the flags.
  \end{itemize}
\end{definition}
The different structures on a graph combine.

\begin{example}
  Let $\mathbf{5} = \{0, 1, 2, 3, 4\}$ be the finite cardinal endowed with the
  order $0 <_{\mathbf{5}} 4$ and $1 <_{\mathbf{5}} 2 <_{\mathbf{5}} 3$, and
  \begin{itemize}
  \item $\Orient_\mathbf{5}$ the orientation defined by
    \begin{align*}
      \Orient_\mathbf{5}(0) &= \Orient_\mathbf{5}(4) = \Out &
      \Orient_\mathbf{5}(1) &= \Orient_\mathbf{5}(2) = \Orient_\mathbf{5}(3) = \In,
    \end{align*}
  \item $\VertType_\mathbf{5}$ defined by $\VertType_\mathbf{5}(\ast) = \maltese$,
  \item $\FlagType_\mathbf{5} \colon \mathbf{5} \to \{a_0,\ldots,a_4\}$ the coloring defined by
    \begin{align*}
      \forall i \in \mathbf{5}, \ \mathsf{c}(i) = a_i.
    \end{align*}
  \end{itemize}
  The ordered labelled oriented colored corolla
  $(\ast_{\mathbf{5}}, \Orient_\mathbf{5}, \VertType_\mathbf{5}, \FlagType_\mathbf{5}, <_{\mathbf{5}})$ is depicted as in Figure \ref{fig:corolla5}.
\end{example}

Each enrichment of the structure of graphs of \Cref{def:labelled-graphs}
induces a notion of morphism that preserves such a structure and an associated category.
For instance, a morphism $h \colon (\tau, \Orient_\tau) \to (\sigma, \Orient_\sigma)$ where $(\tau, \Orient_\tau)$ and $(\sigma, \Orient_\sigma)$ are ordered graphs is such that $\Orient_\sigma \circ h_F = \Orient_\tau$.

We can depict graphs as two-dimensional figures. As a graph is just a
disjoint union of corollas glued with the involution, we only need to show
depictions of corollas (as in \Cref{fig:corolla5}) and how to depict an edge to
be able to depict full graphs. We will always depict the inputs of a corolla
above the corolla, and its outputs below, with arrows also indicating the
orientation. The colors are written next to the arrows. If ordered, the
different flags of a corolla are depicted increasing from left to right.

\begin{figure}[h]
  \centering
  \tikzsetnextfilename{images/corolla}
  \pnet{
    \pnsomenet[t]{$\maltese$}{1.5cm}{0.75cm}
    \pnoutfrom{t.-120}{0}
    \pnoutfrom{t.-45}{4}
    \pninto{t.120}{1}
    \pninto{t.80}{2}
    \pninto{t.45}{3}
  }
  \caption{One depiction of a labelled oriented corolla}
  \label{fig:corolla5}
\end{figure}

\subsection{Trees and paths}
\label{subsec:trees}

%A graph can be realized geometrically. The geometric realization of a
%corolla $\ast_S$ is the disjoint union $\bigsqcup_S [0;\frac{1}{2}]$ with
%end-points $0$ identified. The geometric realization of a graph is the disjoint
%union of the geometric realization of the corollas of all its vertices, with
%points $\frac{1}{2}$ of any two flags forming an orbit under the involution of
%the graph identified.
%
%A graph is \emph{(simply) connected} if its geometric realisation is (simply)
%connected.
%
%A \emph{tree} is a connected, simply connected graph. \index{tree}
%
%
%A \emph{rooted tree} is an oriented tree such that each vertex has exactly one
%$\Out$ flag. A rooted tree only has one output tail. Its boundary is called the
%\emph{root} of the rooted tree.
An \emph{unoriented path} on a graph $\tau$ is a finite sequence of flags $(f_1, \dots, f_{2n})$ for some $n \in \Nat$ such that, for all
$1 \leqslant i \leqslant n$, $j_\tau(f_{2i-1}) = j_\tau(f_{2i})$ and (if $i \neq n$) $\partial_\tau(f_{2i}) = \partial_\tau (f_{2i+1})$. 
Such a path is said to be \emph{between $\partial_\tau(f_1)$ and $\partial_\tau(f_{2n})$} if $n > 0$ (and it is a \emph{cycle} if moreover $\partial_\tau(f_1) =\partial_\tau(f_{2n})$), otherwise it is the \emph{empty path}, which is between any vertex and itself.
Two vertexes $v$ and $v'$ are \emph{connected} if there is an unoriented path between them.

Let $\tau$ be a graph: $\tau$ is \emph{connected} if any vertices $v, v' \in V_\tau$ are connected;
a \emph{connected component} of $\tau$ is a maximal (with respect the inclusion of flags and vertices) connected sub-graph of $\tau$;
$\tau$ is \emph{acyclic} (or a \emph{forest}) if %there is no vertex $v \in V_\tau$ such that there is an unoriented path $(f_1, \dots, f_{2n})$ between $v$ and itself with $n > 0$. 
has no cycles;
$\tau$ is a \emph{tree} if it is a connected forest.

A \emph{rooted tree} is an oriented tree such that each vertex has exactly one
$\Out$ flag. 
A rooted tree has then exactly one output tail: its boundary is called the
\emph{root} of the rooted tree.
A \emph{forest of rooted trees} is a forest whose connected components are rooted trees (and the roots of such trees are the \emph{roots} of the forest).

%A special class of morphism is of interest for rooted trees.
%
%\begin{definition}
%  Let $\tau_1$ and $\tau_2$ be two rooted trees, and $h : \tau_1 \to \tau_2$ be a
%  morphism of graphs.
%  
%  $h$ is a \emph{morphism of rooted trees} if $h_V$ maps the root of $\tau_1$
%  to the root of $\tau_2$. 
%\end{definition}
\begin{remark}
	Let $\tau_1$ and $\tau_2$ be two rooted trees, and $h \colon \tau_1 \to \tau_2$ be a
	morphism of oriented graphs.
	As $h_F$ preserves tails and orientation, $h_V$ maps the root of $\tau_1$ to the root of $\tau_2$. 
\end{remark}

%A \emph{sub-rooted tree} of a tree $\tau$ is a tree $\tau'$ together with an injective morphism of rooted tree $\tau' \to \tau$.  
%It is %sometimes useful to consider %not a rooted tree, but its \emph{reflexive-transitive closure}. 
%the \emph{reflexive-transitive closure} of a rooted tree.
%An (oriented) \emph{path} on a oriented graph $\tau$ is either empty or a sequence $(f_0, \dots, f_{2n+1})$ such that, for all
%$0 \leqslant i < n$, $f_{2i}$ is output and the $f_{2i+1}$
%is input, and  $\partial(f_{2i+1}) = \partial (f_{2i+2})$. Such a
%path is said to be from $\partial(f_0)$ to $\partial(f_{2n+1})$. The empty path
%is a path from any vertex to itself.
%An \emph{oriented path} on a oriented graph $\tau$ is a sequence $(f_1, \dots, f_{2n})$ for some $n \in \Nat$ such that, for all
%$1 \leqslant i \leqslant n$, $f_{2i-1}$ is output, $f_{2i}$
%is input, $j_\tau(f_{2i-1}) = j_\tau(f_{2i})$ and (if $i \neq n$) $\partial_\tau(f_{2i}) = \partial_\tau (f_{2i+1})$. 
%%Such a path is said to be \emph{from $\partial(f_1)$ to $\partial(f_{2n})$}. 
%%The \emph{empty path} is a path from any vertex to itself.
%Such a path is said to be \emph{from $\partial_\tau(f_1)$ to $\partial_\tau(f_{2n})$} if $n > 0$, otherwise it is the \emph{empty path}, which is from any vertex to itself.

An \emph{oriented path} on a oriented graph $\tau$ is an unoriented path $(f_1, \dots, f_{2n})$ for some $n \in \Nat$ such that $f_{2i-1}$ is output and $f_{2i}$ for all $1 \leqslant i \leqslant n$.
Such a path is said to be \emph{from $\partial_\tau(f_1)$ to $\partial_\tau(f_{2n})$} if $n > 0$, otherwise it is the \emph{empty path}, which is from any vertex to itself. 

The set of oriented paths on an oriented tree is finite. 
As such, given a tree $\tau$, we define
its \emph{reflexive-transitive closure}, or \emph{free category},
$\tau^{\circlearrowleft}$ as the oriented graph with same vertices and same tails as $\tau$, and with an edge from $v$ to $v'$ for any oriented path from $v$ to $v'$ in $\tau$.
%more precisely, $\In_{\tau^\circlearrowleft} = \In_{\tau} \{f \mid \}$

Rooted trees and morphisms of rooted tree form a category
$\RootedTree$. The reflexive-transitive closure operator extends to a functor
$(\cdot)^{\circlearrowleft} : \RootedTree \to \CatFont{Graph}$.

%\begin{definition}[Forest, morphism of forests]
%  A \emph{forest} is a set of rooted tree.\footnotemark
%  \footnote{From now on, we identify a set of trees and the graph}
%  A \emph{morphism of forests}
%  $\{\tau_j \mid j \in J\} \to \{\tau'_i \mid i \in I\}$ is a set of rooted tree morphisms $\{\tau_j \to \tau'_j \mid j \in J\}$ where $J \subseteq I$.
%\end{definition}

\subsection{Proof-structures}

\begin{definition}[Module, proof-structure]
  A ($\DiLL$) \emph{module}
  $M = (\rvert M \lvert, \VertType, \Orient, \FlagType,\leqslant)$ is a labelled
  ($\VertType$) oriented ($\Orient$) colored ($\FlagType$) ordered ($\leqslant$)
  graph ($\lvert M \rvert$) such that:
  \begin{itemize}
  \item
    $\VertType \colon V_{|M|} \to \{ \ax, \cut, \One, \bot, \otimes, \parr, \wn,
    \oc\} \cup \{\maltese_p \mid p \in \Nat\}$;
  \item $\FlagType \colon F_{|M|} \to \Formulas_{\MELL}$;
  \item $\leqslant$ is a total order on the flags of $|M|$; the strict order
    associated with it is $<$;
  \item for every $v \in V_{|M|}$,
    \begin{itemize}
    \item if $\VertType(v) = \cut$, the corolla $\tau_v$ has exactly two flags $i_1$
      and $i_2$ which are inputs, and such that
      $\FlagType(i_1) = \FlagType(i_2)^{\bot}$ ;
    \item if $\VertType(v) = \ax$, the corolla $\tau_v$ has exactly two flags $o_1$
      and $o_2$ which are outputs, and such that$
      \FlagType(o_1) = \FlagType(o_2)^{\bot}$;\footnotemark
      \footnotetext{Unlike \cite{PaganiTasson2009}, proof-structures here are
        more general, they need not be with atomic axioms or cut-free.}
    \item if $\VertType(v) \in \{\One, \bot\}$, the corolla $\tau_v$ has no
      inputs and one output $o$, such that $
      \FlagType(o) = \VertType(v)$;
    \item if $\VertType(v) \in \{ \otimes, \parr \}$, the corolla $\tau_v$ has
      exactly two inputs $i_1 < i_2$ and one output $o$, such that
      $\FlagType(o) = \FlagType(i_1) \, \VertType(v) \, \FlagType(i_2)$;
    \item if $\VertType(v) \in \{\wn, \oc\}$, the corolla $\tau_v$ has inputs
      $i_1, \ldots, i_n$ (for some $n\geqslant 0$) and one output $o$, such
      that
      $\forall 1\leqslant j \leqslant n, \ \FlagType(o) = \VertType(v) \,
      \FlagType(i_j)$;\footnotemark \footnotetext{This implies that
        $\FlagType(i_j) = \FlagType(i_k)$ for all
        $1 \leqslant j,k \leqslant n$.}
    \item if $\VertType(v) = \maltese_p$, the corolla $\tau_v$ has no inputs and
      $p \geqslant 0$ outputs $o_1,\ldots,o_p$.\footnotemark 
      \footnotetext{Note that there are conditions on the types of $o_1,\ldots,o_p$.}
    \end{itemize}
    These corollas are depicted \Cref{fig:resource-cells}.
  \end{itemize}
  
  A (\DiLL) \emph{quasi-proof-structure} is a tuple
  $R =(|R|, \TreeT,\BoxFunction)$, where
  $|R| = (\lVert R \rVert, \FlagType_{R}, \Orient_{R}, \VertType_{R},
  \leqslant_{R})$ is a module with no input tails, called the \emph{structured
    graph} of $R$ (and $\lVert R \rVert$ is the \emph{graph} of $R$).
  Moreover, the following conditions are fulfilled:
  \begin{itemize}
  \item $\TreeT$ is a forest of rooted trees with no input tails, called the
    \emph{box-forest} of $R$.
  \item $\BoxFunction \colon |R| \to \TreeT^{\ReflexiveTransitive}$ is a
    morphism of oriented graphs, the \emph{box-function} of $R$, such that,
    for all vertex $v \in V_{|R|}$ with $f \in \In_{|R|}(v)$: % and non-tail:
    \begin{itemize}
    \item if
      $\BoxFunction_V(\partial_{|R|} \circ j_{|R|}(f)) \neq
      \BoxFunction_V(\partial_{|R|}(f))$ then
      $\VertType(v) \in \{ \oc, \wn\}$;
    \item if $\VertType(v) = \oc$ and $\BoxFunction_F(f)$ is a flag of
      $\TreeT$ then
      $\BoxFunction_V(\partial_{|R|}\circ j_{|R|}(f)) \neq
      \BoxFunction_V(\partial_{|R|}(f))$;
    \item $\BoxFunction_F$ induces a partial bijection from
      $\bigcup_{ v \in V_{|R|}, \VertType(v) = \oc}\In_{|R|}(v)$ to the input flags in $\TreeT$.
    \end{itemize}
    
  \item the output tails of $|R|$ are the \emph{conclusions} of $R$; the
    \emph{\MELL conclusion} of $R$ is the list of lists of \MELL formulas
    $(\FlagType(f_1), \dots, \FlagType(f_{i_1}); \cdots ;
    \FlagType(f_{i_{m-1}+1}), \dots, \FlagType(f_n))$ such that
    $\{f_1, \dots, f_n\}$ is the set of conclusions of $R$ with
    $f_i < f_{i+1}$ for all $1 \leqslant i < n$, and
    $0 = i_0 < i_1 < \dots < i_m = n$ and $\Root_1, \dots, \Root_m$ are
    exactly the roots in $\TreeT$, where
    $\BoxFunction_V^{-1}(\Root_{j+1}) = \{\partial_{|R|}(f_{i_{j}+1}), \dots,
    \partial_{|R|}(f_{i_{j+1}})\}$ for all $0 \leqslant j < m$.
    % \item \textbf{ALTERNATIVE:} the output tails of $|R|$ are the
    %   \emph{conclusions} of $R$. The set of the $m\geq 1$ roots of $\TreeT$
    %   yields a partition of $R$'s conclusions in $m$ sets:\\
    %   $\gamma_{\Root}=\{f:\ f\textrm{ is a conclusion of } R\textrm{ and
    % }\partial_{|R|}(f)\in\BoxFunction_V^{-1}(\Root)\}$, where $\Root$ is a
    %   root of $\TreeT$. The order on $R$'s conclusions naturally associates with
    %   $\gamma_{\Root}$ the list $(f^{\Root}_{1}\ldots f^{\Root}_{i_{\Root}})$ of
    %   its elements following this order. And the order on $R$'s conclusions
    %   induces also a total order on $\TreeT$'s roots:
    %   $\Root<_{\TreeT}\Root'\iff min\{f:\ f\textrm{ is a conclusion of }
    %   R\textrm{ and }\partial_{|R|}(f)\in\BoxFunction_V^{-1}(\Root)\}<min\{f:\
    %   f\textrm{ is a conclusion of } R\textrm{ and
    % }\partial_{|R|}(f)\in\BoxFunction_V^{-1}(\Root')\}$, which allows to
    %   naturally associate with the set of the $m$ roots of $\TreeT$ the list
    %   $(\Root_1,\ldots,\Root_m)$. The \emph{\MELL conclusion} of $R$ is the list
    %   of lists of \MELL formulas $\Gamma_{1};\ldots;\Gamma_{m}$, where, for
    %   $1\leq j\leq m$,
    %   $\Gamma_{j}=(\FlagType(f^{j}_{1})\ldots\FlagType(f^{j}_{i_{j}}))$, and
    %   $(f^{j}_{1}\ldots f^{j}_{i_{j}})$ is the list associated with
    %   $\gamma_{\Root_{j}}$.		
  \end{itemize}
  
  A $\MELL$ \emph{quasi-proof-structure} is a quasi-proof-structure such that:
  \begin{itemize}
  \item for all $v \in V_{|R|}$, if $\VertType(v) = \oc$ then
    $\Card{\In_{|R|}(v)} = 1$;
  \item the bijection induced by $\BoxFunction_F$ from
    $\bigcup_{ v \in V_{|R|}, \VertType(v) = \oc}\In_{|R|}(v)$ to the input
    flags in $\TreeT$ is total.
  \end{itemize}
  A $\DiLL_0$ \emph{quasi-proof-structure} (or \emph{polyadic
    quasi-proof-structure}) is a quasi-proof-structure such that its
  box-forest is just a juxtaposition %set
  of roots.
  
  A ($\DiLL$) \emph{proof-structure} is a quasi-proof-structure whose
  box-forest is a tree.  A $\MELL$ (resp.~$\DiLL_0$ or \emph{polyadic})
  \emph{proof-structure} is a proof-structure which is a $\MELL$
  (resp.~$\DiLL_0$) quasi-proof-structure.
\end{definition}

Let $R = (|R|, \TreeT_{R}, \BoxFunction_{R})$ be a quasi-proof-structure.  With
every flag of $|R|$ such that ${\BoxFunction_{R_F}}(f)$ is an input flag of
$\TreeT_{R}$\footnotemark \footnotetext{According to the constraints on
  $\BoxFunction_{R}$, this condition can be fulfilled only by inputs of a
  $\oc$-cell in $|R|$, and an input of a $\oc$-cell need not fulfill it; in
  particular, if $R$ is a \MELL quasi-proof-structure, then this condition is
  fulfilled by all and only the inputs of $\oc$-cells (and such a input is
  unique for every $\oc$-cell) in $|R|$; but if $R$ is a $\DiLL_0$
  quasi-proof-structure, then this condition is not fulfilled by any flag in
  $|R|$ (since $\TreeT_{R}$ has no inputs) and so $\BoxFunction_{R}$ is a graph
  morphism associating a root of $\TreeT_{R}$ with every vertex of $|R|$.
  Therefore, for a $\DiLL_0$ quasi-proof-structure
  $R = (|R|,\TreeT_{R},\BoxFunction_{R})$, the structure induced by $\TreeT_{R}$
  and $\BoxFunction_{R}$ on $|R|$ is just a partition of the list of the types
  of the conclusions of $|R|$.}  there is associated a \emph{box}, that is the
subgraph of $|R|$ made up of all the vertexes $v$ such that there is an oriented
path on $\TreeT_{R}$ from ${\BoxFunction_{R_V}}(v)$ to
${\BoxFunction_{R_V}}(\partial_{|R|} \circ j_{|R|}(f))$.  Thus, every non-root
vertex of $\TreeT_{R}$ represents a box in $R$, and the roots of $\TreeT$
represent the parts of $R$ outside all the boxes.

The quasi-proof-structures we have just defined are particularly rigid: a
proof-structure is dependent on its carrier-sets of cells and wires.  We will
only consider quasi-proof-structures modulo the isomorphism arising from its
labelled graph structure.

\begin{definition}[Isomorphism of proof-structures]
	\label{def:iso}
	Let $R = (|R|, \TreeT_{R}, \BoxFunction_R)$ and $R' = (|R'|, \TreeT_{R'},\allowbreak \BoxFunction_{R'})$ be quasi-proof-structures, with $|R| = (\lVert R \rVert, \VertType_{R}, \Orient_{R}, \FlagType_{R}, \leqslant_{R})$ and $|R'| = (\lVert R' \rVert, \VertType_{R'}, \Orient_{R'},\allowbreak \FlagType_{R'}, \leqslant_{R'})$.
  An \emph{isomorphism of quasi-proof-structures} $f \colon R \simeq R'$ is
  \begin{itemize}
  \item an isomorphism $f \colon (\lVert R \rVert, \VertType_{R}, \Orient_{R}, \FlagType_{R}) \to (\lVert R' \rVert, \VertType_{R'}, \Orient_{R'},\allowbreak \FlagType_{R'})$ of the %underlying 
  structured graphs of $R$ and $R'$ (except $\leqslant_R$ and $\leqslant_{R'}$),
  \item an isomorphism $f_{\BoxFunction} \colon \TreeT_{R} \to \TreeT_{R'}$ of the box-forests of $R$ and $R'$,
  \end{itemize}
  such that the following diagram commutes
  \tikzsetnextfilename{images/proof-net-isomorphism}
  \begin{commutativediagram}{5}{5}{5}
    {
      {|R|} \& \TreeT_R^{\ReflexiveTransitive}\\
      {|R'|} \& \TreeT_{R'}^{\ReflexiveTransitive}\\
    };
    \path[-stealth]
    (m-1-1) edge [auto] node {$\BoxFunction_R$} (m-1-2)
    (m-1-1) edge [auto] node {$f$} (m-2-1)
    (m-1-2) edge [auto] node {$f_{\BoxFunction}^{\ReflexiveTransitive}$} (m-2-2)
    (m-2-1) edge [auto] node {$\BoxFunction_{R'}$} (m-2-2);
  \end{commutativediagram}
%  \noindent and such that, moreover, the restrictions of $f$ on:
%  \begin{itemize}
%  \item the tails,
%  \item the inputs of each cell of type $\wn, \otimes, \parr$,
%  \end{itemize}
%  are all increasing.
		\noindent and moreover each restriction of $f$ on:
		\begin{itemize}
			\item the %tails,
			conclusions of $R$,
			\item the inputs of each cell of type $\oc, \wn, \otimes, \parr$,
		\end{itemize}
		preserves the order $\leqslant_{R}$ (on $\leqslant_{R'}$).
\end{definition}

%We will actually
We shall always consider quasi-proof-structures \emph{up to this isomorphism},
and shall implicitly verify that any construction factors through the quotient
induced by this isomorphism.  Note that if $R$ is isomorphic to a
quasi-proof-structure $R'$, and $R$ is a proof-structure, or a \MELL or
$\DiLL_0$ quasi-proof-structure, then $R'$ is a proof-structure, or a \MELL or
$\DiLL_0$ quasi-proof-structure, respectively.

\begin{remark}
  Differently from us, \DiLL, \MELL and $\DiLL_0$ proof-structures are usually
  defined without an order in the inputs of a $\oc$- or $\wn$-cell.  Such a
  standard definition can be recovered in our setting by just slightly modifying
  the definition of isomorphism (Def.\ref{def:iso}).  First, we replace the
  condition of the restrictions of $f$ with "each restriction of $f$ on:
  \begin{itemize}
  \item the conclusions of $R$ (this condition is dropped if we want to
    define proof-structures without an order in their conclusions),
  \item the inputs of each cell of type $\otimes, \parr$,
  \end{itemize}
  preserves the order $\leqslant_{R}$ (on $\leqslant_{R'}$)".
  
  Then, we say that a \emph{standard \DiLL} (resp.~\MELL; $\DiLL_0$)
  \emph{proof-structure} is an equivalence class of \DiLL (resp.~\MELL;
  $\DiLL_0$) proof-structures through isomorphisms of quasi-proof-structures.
\end{remark}
