# Supplementary material for: Glueability of resource proof-structures: inverting the Taylor expansion (long version)
Source: arXiv:1910.07936 source file (2019-10-17)
Supplement: Supplementary file 2 [file taylor-appendix.tex]

\section{Formal definitions of the fattened Taylor expansion}
\label{sec:taylor-appendix}

\begin{lemma}
  \label{lem:cell-in-taylor-to-mell}
  Let $R$ be a $\MELL$ quasi-proof-structure and $\rho$ in the Taylor expansion
  of $R$.
  If there is a cell of type $\ell \neq \maltese$ rooted in $i$ in $\rho$, then,
  there is a $\ell$-cell rooted in $i$ in $R$.
\end{lemma}

Given $R =(|R|, \TreeT_{R},\BoxFunction_{R})\in\qMELL$, the set of all $\MELL$
quasi-proof-structures and $r$ root of $\TreeT_{R}$, we can define the $\MELL$
proof-structure $R_{r}=(|R_{r}|, \TreeT_{R_{r}},\BoxFunction_{R_{r}})$. If we
call $Root_{\TreeT}$ the set of roots of the forest $\TreeT$, the $\qMELL$
proof-structure $R$ can be defined as the set
$\{R_{r}:\ r\in Root_{\TreeT_{R}}\}$.

Given an upward-closed set of cells $S$ in a forest $\TreeT$, we write:
\begin{itemize}
\item $S^{\circ}$ for the set of cells of $S$ such that, for every
  $v\in S^{\circ}$, there exists a cell $v'\in S$ such that $v'\neq v$ and $v'$
  is below $v$ in $\TreeT$
\item $\partial S = S\setminus S^{\circ}$
\item $\TreeT^S$ for the forest obtained by removing from $\TreeT$ the cells of
$S^{\circ}$.
\end{itemize} Note that the roots of $\TreeT^S$ are the same as the roots of
$\TreeT$.

\begin{definition}[emptying]
  Let $R =(|R|, \TreeT,\BoxFunction)\in\MELL$\footnote{Remember that, since $R\in\MELL$, $\TreeT$ is a tree and has thus a unique root.}, let $S$ be an upward-closed
  set of cells in $\TreeT$, let $k \geq 0$ and $i_1,\dots,i_k$ be conclusions
  of $R$ such that, for $j\in\{1,\ldots,k\}$, $\partial_{|R|}(i_{j})=v_{j}$ is a $\wn$-cell and $\BoxFunction_{V}(v_{j})\in S$\footnote{Notice that since $i_{j}$ is a conclusion of $R$ necessarily $\BoxFunction_{V}(v_{j})$ is the root of $\TreeT$, so $\BoxFunction_{V}(v_{j})\in S$ is equivalent to say that the root of $\TreeT$ is an element of $S$, that is $\TreeT=S$.}.
  
   The \emph{emptying} of $R$ relatively to $S$ and $i_1,\dots,i_k$ is the
  $\MELL$ proof-structure $R^S_{i_1,\dots,i_k}=(|R^{S}_{i_1,\dots,i_k}|,
  \TreeT^S,\BoxFunction^S)$ defined by\footnote{Notice that when $S=\emptyset$ we have $R^S_{i_1,\dots,i_k}=R$.}:
  \begin{itemize}
  \item if the root of $\TreeT$ is in $S$ (that is $\TreeT=S$), then $\TreeT^S$ is reduced to this root $\bullet$.

    Let $p=m+\Sigma_{1\leq j\leq n}m_{j}$, where for $j\in\{1,\ldots,k\}$ $v_{j}=\partial_{|R|}(i_{j})$ has $m_j$ premises and $m$ is the number of conclusions of $R$ different from $i_1,\dots,i_k$.

    We set $V_{|R^{S}_{i_1,\dots,i_k}|}=\{v\}\cup\{v_{1},\ldots,v_{k}\}$, where
    $\VertType(v)=\maltese_{p}$ and
    $\BoxFunction^S_{V}(v)=\BoxFunction^S_{V}(v_{j})=\bullet$ (for $1\leq j\leq k$).
  \item if the root of $\TreeT$ is not in $S$ (that is $\TreeT\neq S$), we have $\BoxFunction_{V}(\partial_{|R|}(i))\not\in S$ for every conclusion $i$ of $R$, so that there are no conclusions
    $i_1,\dots,i_k$ and we forego them in the notations.

    We set $V_{|R^{S}_{i_1,\dots,i_k}|}=V\cup V^{+}$, where
    $V=\{v\in V_{R}:\ \BoxFunction_{V}(v)\in\TreeT^{S} \setminus
    \partial S\}$ and $V^{+}=\{v_{1},\ldots,v_{k}\}$, where
    $\partial S=\{s_{1},\ldots,s_{k}\}$ and, for every $i\in\{1,\ldots,k\}$,
    $\VertType(v_{i})=\maltese_{p_{i}}$ with
    $p_{i}=card(\{f\in F_{|R|}:\ \BoxFunction_{F}(f)\textrm{ is the unique
      output of }s_{i}\textrm{ in }\TreeT\}$. Then we set:
    \begin{itemize}
    \item $\BoxFunction^S_{V}(v)=\BoxFunction_{V}(v)$ for $v\in V$;
    \item $\BoxFunction^S_{V}(v_{i})=s_{i}$ for $i\in\{1,\ldots,k\}$.
    \end{itemize}
  \end{itemize}

  We then define the emptying in $\qMELL$ component by component.
\end{definition}

\begin{lemma}
  \label{lem:cell-in-mell-to-emptying}

  Let $R$ be a $\MELL$ quasi-proof-structure and $R^S$ be one of its emptying.

  If there is a cell of type $\ell \neq \maltese$ rooted in $i$ in $R^S$, then,
  there is a $\ell$-cell rooted in $i$ in $R$.
\end{lemma}
\begin{proof}
  Let $i$ be a conclusion of $R$, and $c$ its attached cell. Suppose that the
  type of the cell attached to $i$ in $R^S$ is $\ell \neq \maltese$.

  If the image $b$ of $c$ in the box-forest of $R$ is not in $S$, then $b$ is
  also present in $\TreeT^S$ and its inverse image through $\BoxFunction_{R^S}$
  is the same as the inverse image of $b$ through $\BoxFunction_R$, so in
  particular $c$ has type $\ell$.

  Else, the inverse image of $b$ through $\BoxFunction_{R^S}$ contains only
  $\maltese$ and $\wn$-cells. So, the only possibility left is that $\ell =
  \wn$. The $\wn$-cells are placed on $R^S$ only as conclusions in which a
  $\wn$-cell is rooted in $R$. Hence the lemma.
\end{proof}

\begin{definition}[$S$-fat]
  Let $R =(|R|, \TreeT,\BoxFunction)$ be a $\qMELL$ proof-structure and $S$ be an upward-closed
  set of cells in $\TreeT$.
  
  A thick subtree $t = (\tau_t, h_t)$ of $\TreeT^S$ is said \emph{$S$-fat} if:
  \begin{itemize}
  \item $h_{t}$ is surjective on $\TreeT^S \setminus \partial S$;
  \item for every $s \in \partial S$, either $s$ is a root, in which case we ask that 
    $h_{t}^{-1}(s)$ is a singleton, or $s$ has an immediate ancestor (its father) $b$ in
    $\TreeT^S$, and in this case we ask that the two following sets of vertices of $\tau_t$ have the same number of elements: $h_{t}^{-1}(b)$ and $h_{t}^{-1}(s)$.
      \end{itemize}

  The \emph{fattened Taylor expansion} of $R$ is the set\footnote{Notice that when $S=\emptyset$ we have $\TreeT^S=\TreeT$, $R=R^{S}$, the $\emptyset$-fat thick subtree $t = (\tau_t, h_t)$ of $\TreeT^S$ is a fat subtree of $\TreeT$ such that there are no cells of type $\maltese$ in $\tau_t$: in this case $(R^S_t, [\tau_t], \overline{h_t})=(R_t, [\tau_t], \overline{h_t})$ is an element of the Taylor expansion of $R$.}
  \[\{ (R^S_t, [\tau_t], \overline{h_t}) \mid S \text{ upwards closed set of cells of } \TreeT, t~S\text{-fat
    thick subtree of } \TreeT^S\}.\]
\end{definition}

\begin{proposition}
If $\rho^{\maltese}$ is in the fattened Taylor expansion of $R\in\qMELL$, then there exists a polyadic quasi-proof-structure $\rho$ such that $\rho^{\maltese}$ is a fattening of $\rho$ and $\rho$ is in the Taylor expansion of $R$.
\end{proposition}

\begin{proof}
  Let $R =(|R|, \TreeT,\BoxFunction)$, let $S$ be an upwards closed subset of
  $\TreeT$, and let $t = (\tau_t, h_t)$ be the thick subtree of $\TreeT^S$ such
  that $(\rho^{\maltese}, [\tau_t], \overline{h_t})$ is in the fattened Taylor
  expansion of $R$. Notice that if $c$ is a $\maltese$-cell of
  $R_{t}=\rho^{\maltese}$, then $h_{t}(p_{tl}((c))\in\partial S$. However, the
  converse does not hold when $\TreeT=S$: one might have a $?$-cell $c$ of
  $R_{t}=\rho^{\maltese}$, such that $h_{t}(p_{tl}((c))$ is the root of $\TreeT$
  (that is $h_{t}(p_{tl}((c))\in\partial S$).

If $\TreeT=S$, let $t'=(\emptyset,\emptyset)$ be the empty thick subtree of
$\TreeT^{S}$. If $\TreeT\neq S$, then $h_{t}(p_{tl}((c))\in\partial S$ iff $c$
is a $\maltese$-cell of $R_{t}=\rho^{\maltese}$, and we set
$\rho=(R_{t'}, [\tau_{t'}], \overline{h_{t'}})$ where $t'=(\tau_{t'}, h_{t'})$
is obtained from $t=(\tau_{t}, h_{t})$ by removing from $\tau_{t}$ all the cells
$p_{tl}((c)$ such that $c$ is a $\maltese$-cell of $R_{t}=\rho^{\maltese}$ and
and $h_{t'}$ is the obvious restriction of $h_{t}$ to $\tau_{t'}$.  In both
cases $t'$ is both a thick subtree of $\TreeT^{S}$ and of $\TreeT$. Thus
$(R_{t'}, [\tau_{t'}], \overline{h_{t'}})$ is an element of the Taylor expansion
of $R$, and $(\rho^{\maltese}, [\tau_t], \overline{h_t})$ is a fattening of
$\rho=(R_{t'}, [\tau_{t'}], \overline{h_{t'}})$.
\end{proof}

\begin{lemma}
  \label{lem:connexity-mell-to-taylor}
  Let $R$ be a $\MELL$ quasi-proof-structure and $\rho$ in the fattened Taylor
  expansion of $R$.
  Let $i$ and $j$ be two conclusions. If $i$ and $j$ are connected in $R$, they
  are connected in $\rho$.
\end{lemma}

\begin{lemma}
  \label{lem:cell-in-fat-taylor-to-mell}

  Let $R$ be a $\MELL$ quasi-proof-structure and $\rho$ in the fattened Taylor
  expansion of $R$.

  If there is a cell of type $\ell \neq \maltese$ rooted in $i$ in $\rho$,
  then, there is a $\wn$-cell rooted in $i$ in $R$.

  Conversely, if there is a cell of type $\ell$ rooted in $i$ in $R$, there is
  a cell of type either $\ell$ or $\maltese$ in $\rho$.
\end{lemma}
\begin{proof}
  By \Cref{lem:cell-in-taylor-to-mell} and \Cref{lem:cell-in-mell-to-emptying}.
\end{proof}
